# Supplementary material for: High-purity frequency-degenerate photon pair generation via cascaded SFG/SPDC in thin film lithium niobate
Source: arXiv:2512.13248 source file (2025-12-15)
Supplement: Supplementary file 1 [file Supplementary.pdf]

# Supplementary Material for: High-purity frequency-degenerate photon pair generation via cascaded SFG/SPDC in thin film lithium niobate

## 1. MODEL FOR SFG

In this section, we derive the solution of the coupled wave equations (CWEs) of SFG and define its conversion efficiency. In a SFG process, two pumps with angular frequency  $\omega_1$  and  $\omega_2$  interact together to create a third wave at  $\omega_{\text{SF}} = \omega_1 + \omega_2$ . The CWEs describing the evolution of the complex amplitude,  $A(z)$ , are given by:

$$\frac{\partial A_1}{\partial z} = -i\kappa_{\text{SFG},1} A_2(z)^* A_{\text{SF}}(z) e^{-i\Delta k_{\text{SF}} z} \quad (\text{S1})$$

$$\frac{\partial A_2}{\partial z} = -i\kappa_{\text{SFG},2} A_1(z)^* A_{\text{SF}}(z) e^{-i\Delta k_{\text{SF}} z} \quad (\text{S2})$$

$$\frac{\partial A_{\text{SF}}}{\partial z} = -i\kappa_{\text{SFG,SF}} A_1(z) A_2(z) e^{i\Delta k_{\text{SF}} z}, \quad (\text{S3})$$

$$(\text{S4})$$

where  $\Delta k_{\text{SF}} = k_1 + k_2 - k_{\text{SF}}$  is the phase matching and  $k_i$ , with  $i = 1, 2, \text{SF}$  are the wavevectors of the pumps and of the SF. The nonlinear coupling coefficients are defined as

$$\kappa_{\text{SFG},j} = \frac{\sqrt{2}\omega_j d_{\text{eff}}}{c^{3/2} \sqrt{\epsilon_0 n_{\text{SF}} n_1 n_2} A_{\text{eff,SFG}}}, \quad (\text{S5})$$

with  $j = 1, 2, \text{SF}$ . The effective nonlinear coefficient  $d_{\text{eff}}$  is given by 25 pm/V (in the case of MPM and rescaled with a factor of  $(2/\pi)$  in first order QPM). The speed of light, the vacuum permittivity and the effective refractive indices of the modes are denoted with  $c$ ,  $\epsilon_0$  and  $n_j$  with  $j = 1, 2, \text{SF}$ , respectively. The effective area,

$$A_{\text{eff,SFG}} = \frac{\iint |e_1(x, y)|^2 dS \iint |e_2(x, y)|^2 dS \iint |e_{\text{SF}}(x, y)|^2 dS}{\left( \iint_{\chi^{(2)}} e_{\text{SF}}(x, y) e_1^*(x, y) e_2^*(x, y) dS \right)^2}, \quad (\text{S6})$$

is expressed in terms of normalization factors in the numerator and of an overlap integral across the nonlinear cross-section, i.e. where  $|\chi^{(2)}(x, y)| \geq 0$ , between the three mode profiles at the denominator. Here  $e_j(x, y)$  with  $j = 1, 2, \text{SF}$  are the transverse electric field components (TE components) of the modes. Making the undepleted approximations for both pumps, i.e.  $\frac{\partial A_1}{\partial z} = \frac{\partial A_2}{\partial z} = 0$ , the solution for the power of the SFG,  $P_{\text{SF}}(z) = |A_{\text{SF}}(z)|^2$ , is given by:

$$P_{\text{SF}}(z) = \kappa_{\text{SFG,SF}}^2 P_1 P_2 \text{sinc}^2 \left( \frac{\Delta k_{\text{SF}} z}{2} \right). \quad (\text{S7})$$

We define the SFG conversion efficiency ( $\eta_{\text{SFG}}$ ) as:

$$\eta_{\text{SFG}} = \frac{P_{\text{SF}}}{P_1 P_2 L^2} = \kappa_{\text{SFG,SF}}^2 \quad (\text{S8})$$

where  $L$  is the waveguide length and the SF power is evaluated at  $z = L$ .

## 2. MODEL FOR CASCADED SFG/DEGENERATE-SPDC

In this section, we retrieve the scaling law and dependencies of the pair generation rate as a function of the pump powers, of the waveguide length and of the nonlinear conversion efficiency, in the case of cSFG/degenerate-SPDC. Here, we use the classical CWEs and focus on a single frequency pair for SPDC, i.e. the degenerate case when the idler and signal frequency are equal, neglecting all other photon pairs allowed by energy conservation and within the SPDC bandwidth. Indeed, SPDC can be modelled as a DFG process seeded by vacuum fluctuations [1], which can be modelled as a complex Gaussian random variable, with zero mean and a variance of half the photon's energy [2–4]. This approach neglects the thermal excitations [4], the time-dependency of the vacuum fluctuations in different point in space and the other possible photon pairs.

A more accurate semi-classical model for SPDC, could be obtained with a summation on all possible photon pairs allowed by energy conservation within the SPDC bandwidth [2–4].

The amplitudes of the two pumps, of the SFG and of the degenerate idler/signal are denoted with the indices 1, 2, SF and i, respectively. At phase matching for the two processes, where  $\Delta k_{SF} = k_{SF} - k_1 - k_2 = 0$  and  $\Delta k_{DFG} = 2k_i - k_{SF} = 0$ , the CWEs are given by:

$$\frac{\partial A_1}{\partial z} = -i\kappa_{SFG,1} A_2(z)^* A_{SF}(z) \quad (S9)$$

$$\frac{\partial A_2}{\partial z} = -i\kappa_{SFG,2} A_1(z)^* A_{SF}(z) \quad (S10)$$

$$\frac{\partial A_{SF}}{\partial z} = -i\kappa_{SFG,SF} A_1(z) A_2(z) - i\kappa_{DFG} A_i^2(z) \quad (S11)$$

$$\frac{\partial A_i}{\partial z} = -i\kappa_{DFG} A_{SF}(z) A_i^*(z) \quad (S12)$$

The DFG nonlinear coupling coefficient is expressed as:

$$\kappa_{DFG} = \frac{\sqrt{2}\omega_i d_{\text{eff}}}{c^{3/2} \sqrt{\epsilon_0 n_{SF} n_1 n_2} A_{\text{eff},DFG}}. \quad (S13)$$

The conversion efficiency then follows the relation  $\eta_{DFG} = \kappa_{DFG}^2$  and the effective area is given by

$$A_{\text{eff},DFG} = \frac{\left( \iint |e_i(x, y)|^2 dS \right)^2 \iint |e_{SF}(x, y)|^2 dS}{\left( \iint_{\chi^{(2)}} e_{SF}(x, y) (e_i^*(x, y))^2 dS \right)^2}. \quad (S14)$$

The denominator is integrated in the domain where the second order nonlinear susceptibility is nonzero, i.e.  $|\chi^{(2)}(x, y)| \geq 0$ . We make the undepleted approximations for both pumps, i.e.  $\frac{\partial A_1}{\partial z} = \frac{\partial A_2}{\partial z} = 0$ , and neglect the second term in the right-hand side of Eq. 3 as it is much smaller than the first term. We solve Eq. S11 and obtain that

$$A_{SF}(z) = -i\kappa_{SFG,SF} A_1 A_2 z \quad (S15)$$

Substituting Eq. S15 in Eq. S12 gives

$$\frac{\partial A_i}{\partial z} = \gamma z A_i^*(z), \quad (S16)$$

where  $\gamma = -A_1 A_2 \kappa_{SFG,SF} \kappa_{DFG}$  can be made positive and real by an appropriate choice of the phase of the pumps. This equation can be solved by separating the amplitude into its real and imaginary parts,  $A_i(z) = a(z) + ib(z)$ , yielding:

$$\frac{\partial a(z)}{\partial z} = \gamma z a(z) \quad (S17)$$

$$\frac{\partial b(z)}{\partial z} = -\gamma z b(z). \quad (S18)$$

The solution to these equations are  $a(z) = a(0)e^{\frac{\gamma z^2}{2}}$  and  $b(z) = b(0)e^{-\frac{\gamma z^2}{2}}$ . This results in  $A_i(z) = a(0)e^{\frac{\gamma z^2}{2}} + ib(0)e^{-\frac{\gamma z^2}{2}}$ . As the variances of the power in the two quadratures are both equal to the vacuum fluctuations, i.e. to the ground state of a quantum harmonic oscillator

divided by  $T$ , the time bandwidth of the photons,  $|a(0)|^2 = |b(0)|^2 = \frac{\hbar\omega_i}{2T}$  [1, 2]. Thus, the idler power grows as:

$$P_i(z) = a(z)^2 + b(z)^2 = \frac{\hbar\omega_i}{2T} (e^{\gamma z^2} + e^{-\gamma z^2}) = \frac{\hbar\omega_i}{T} \cosh(\gamma z^2) \approx \frac{\hbar\omega_i}{T} (1 + \frac{\gamma^2 z^4}{2}), \quad (\text{S19})$$

where the last approximation assumes that  $\frac{\gamma z^2}{2} \ll 1$ . For short waveguide length  $L$ , we see that the idler power scales with the fourth order of the waveguide length, with the product of the SFG and DFG conversion efficiency and with the product of the pump powers, i.e.

$$P_i(z) \propto L^4 \eta_{\text{SF}} \eta_{\text{DFG}} P_1 P_2 \approx 4L^4 \eta_{\text{SH}}^2 P_1 P_2, \quad (\text{S20})$$

The last approximation holds as the effective area in the SH conversion efficiency is very similar to the one of SFG for small frequency detuning between the two pumps and it is equal to the one of DFG in the degenerate case. Note that there is a factor 2 in the nonlinear coupling coefficient due to the term of the angular frequency, such that  $\kappa_{\text{SFG,SF}} = 2\kappa_{\text{DFG}} = 2\kappa_{\text{SH}}$ .

### 3. DERIVATION OF THE PAIR GENERATION RATE AND COINCIDENTAL TO ACCIDENTAL RATIO

To compute the pair generation rate (PGR) and coincidental to accidental ratio (CAR), we assume that the correlation between the arrival times of the photon pairs follows a gaussian distribution, associated with the detectors jitter (here 50 ps). Then, we apply a gaussian fit to the coincidental histogram. We define the coincidental counts,  $N_{\text{cc}}$ , as the area in the full width at half maximum (FWHM) of the gaussian distribution and the accidental counts,  $N_{\text{acc}}$ , as the area below the floor of the distribution, as illustrated in Fig. S1.

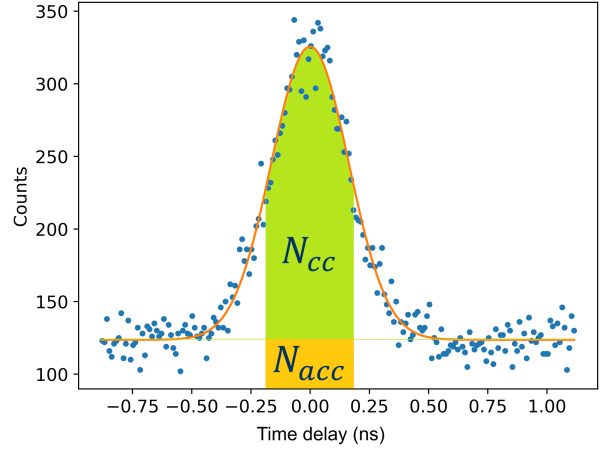

**Fig. S1.** Coincidental histogram from which we infer the coincidental counts,  $N_{\text{cc}}$ , and the accidental counts,  $N_{\text{acc}}$ .

The CAR is defined as:

$$\text{CAR} = \frac{N_{\text{cc}}}{N_{\text{acc}}}. \quad (\text{S21})$$

To obtain the number of on-chip generated pairs,  $N_{\text{cc,on-chip}}$ , we estimate the output coupling losses to 4.8 dB, measure the propagation losses through the CDWM stages and through the waveshaper, the 50:50 BS, the polarization controller and in the fiber guiding light to the superconducting nanowire single-photon detector (SNSPD). We also add a factor to take into account the detection efficiency of the SNSPDs. These losses are added to each channel going to the SNSPDs, separately. Additionally, we need to compensate for 3 dB of losses in the 50:50 BS, due to the fact that, out of 4 outcomes, the photon pairs are sent to the same detector in 2 outcomes. Then the PGR is given by:

$$\text{PGR} = \frac{N_{\text{cc,on-chip}}}{\tau}, \quad (\text{S22})$$

where  $\tau$  is the integration time of the SNSPD. As said in the main text, in the case of DP cSFG/SPDC, we define the normalized brightness as:

$$B = \frac{PGR}{4\Delta\lambda P_1 P_2}, \quad (\text{S23})$$

where  $\Delta\lambda$  is the SPDC measurement bandwidth, given by the tunable waveshaper bandwidth in our experiment, and  $P_{pi}$  with  $i = 1, 2$  are the pump powers. Note that the factor 4 is required to compare the brightness from cSHG/SPDC and cSFG/SPDC. Indeed, SHG is proportional to  $P_p^2$ , while SFG scales with  $4P_1 P_2$ .

#### 4. CONTRIBUTION OF PARASITIC PARAMETRIC PROCESSES TO NOISE

In this section, we theoretically derive the efficiency of the two main parasitic processes that can contribute to lower the CAR of the degenerate photon pairs: Dual-pump Spontaneous Four-Wave Mixing and Single pump cSHG/SPDC processes.

##### A. Four-wave mixing conversion efficiency

In this section, we estimate the conversion efficiency of four-wave mixing (FWM) in our single-pass waveguides. We start by the non-degenerate case, with two incoming pumps. Neglecting the depletion of the pumps and of the signal (meaning their power remain constant along the propagation length), neglecting further the propagation losses and assuming phase matching, i.e.  $\Delta\beta = \beta_1 + \beta_2 - \beta_s - \beta_i = 0$ , where  $\beta_j$  with  $j = p1, p2, s, i$  are the wavevectors of the pumps, of the signal and of the idler, then the power of the idler can be approximated by [5]:

$$P_i(L) = 4\gamma^2 P_1 P_2 P_s L^2. \quad (\text{S24})$$

Here  $L$  is the length of the waveguide and  $\gamma = k_0 n_2 / A_{\text{eff}}$ , where  $k_0 = \frac{2\pi}{\lambda_0}$  with  $\lambda_0$  the vacuum wavelength,  $A_{\text{eff}}$  is the effective area of the propagating mode and  $n_2$  is the nonlinear refractive index, which is worth  $1.8 \times 10^{-19} \text{ m}^2 \text{ W}^{-1}$  in LN [6].

Since having a single pump with a power  $P_p$  or two pumps with a power  $P_1 = P_2 = \frac{P_p}{2}$  should generate an equivalent amount of power for the idler, due to energy conservation, we divide the power of the pumps by 2 in Eq. S24 to obtain the equivalent approximation in the degenerate case (with a single pump):

$$P_i(L) = 4\gamma^2 \left(\frac{P_p}{2}\right)^2 P_s L^2 = \gamma^2 P_p^2 P_s L^2. \quad (\text{S25})$$

This formula is consistent with the degeneracy factor of 6 (3), involved in the nonlinear polarization, due to the permutation of the 3 (2) incoming waves driving the nonlinear polarization in the non-degenerate (degenerate) case.

Our waveguide is  $L = 4.45 \text{ mm}$  long and has  $A_{\text{eff}} = 0.736 \mu\text{m}^2$ . Then, using Eq. S25, we get  $\frac{P_i(L)}{P_p^2 P_s} = 1.95 \times 10^{-5} \text{ W}^{-2}$ . With 1 mW of pump power and the vacuum fluctuations for the signal ( $\sim 3 \times 10^{-8} \text{ W}$ ), only  $\sim 5.8 \times 10^{-19} \text{ W}$  of idler would be generated. This is why FWM requires field enhancement in microresonators to become efficient.

##### B. cSHG/DFG conversion efficiency

An analytical solution of cSHG/DFG can be found in [7]. Here, to estimate the cSHG/DFG conversion efficiency away from phase matching, we simulate its CWEs with low pump of 1 mW, to remain in the undepleted pump regime. We use  $L = 4.45 \text{ mm}$  and the second-order nonlinear coefficient  $d_{33} = 25 \text{ pm/V}$ . In the simulation, we rescale the coupling coefficients to enforce the experimental conversion efficiency of  $250 \% \text{ W}^{-1} \text{ cm}^{-2}$ . The initial conditions of the idler, signal and SH powers are given by the vacuum fluctuations. For the signal and idler, we set  $P_i(0) = P_s(0) = \frac{\hbar\omega_i}{T} = 3 \times 10^{-8} \text{ W}$ , where  $T = \frac{1}{\Delta f} = \frac{\lambda^2}{c\Delta\lambda} = 4 \text{ ps}$  is the time-bandwidth of the photon (considering  $\Delta\lambda = 2 \text{ nm}$ ). For the SH, using the same formula, we set  $P_{\text{SH}}(0) = 2.7 \times 10^{-7} \text{ W}$ .

We simulate cSHG/DFG by placing the signal at phase matching and red-detune the pump by 20 nm, to simulate the parasitic process at degeneracy in the same configuration than in the DP experiment.

Fig. S2 a) shows that the SH power oscillates along the propagation direction  $z$  as a result of phase mismatch. This behavior arises because the phase difference between the SH wave and the pump accumulates over distance. When the phase difference is shifted by  $\pi$ , the direction of energy transfer reverses: from the pump to the SH, and then back. Consequently, the power of the SH undergoes periodic cycles of amplification and deamplification, a phenomenon often referred to as back-conversion and prevent a consistent amplification of the signal and idler. At most, the idler power increases only by  $\Delta P_i = 4 \times 10^{-7} \mu\text{W}$  from its initial condition but does not coherently accumulate. It is 6 order of magnitude higher than FWM so this suggest that the main contribution of the histogram in Fig. 3 f) in the main text, originates from cSHG/DFG rather than degenerate SFWM.

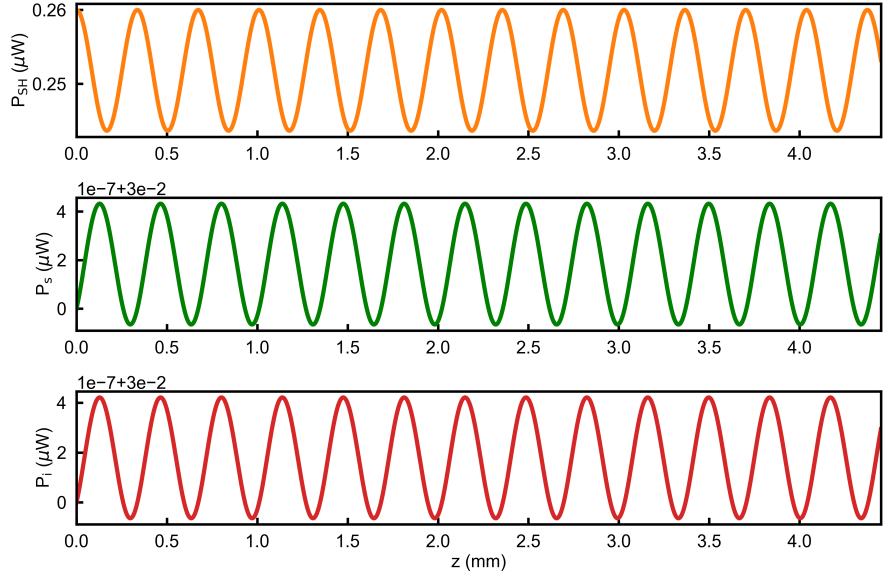

**Fig. S2.** cSHG/DFG simulation where the SHG pump is detuned by 20 nm from the phase matching wavelength. Due to phase mismatch, the SHG power oscillates along the waveguide. When the relative phase between the pump and the SH wave reaches  $\pi$ , the direction of energy flow reverses, transferring energy back from the SH to the pump. A similar behavior is observed for the signal and idler waves. Over a 1 mm propagation length, three full cycles of energy transfer between the SHG pump and the SH wave occur, and the idler power remains negligible.

## REFERENCES

1. L. G. Helt, M. Liscidini, and J. E. Sipe, "How does it scale? comparing quantum and classical nonlinear optical processes in integrated devices," *J. Opt. Soc. Am. B* **29**, 2199–2212 (2012).
2. A. Fix and R. Wallenstein, "Spectral properties of pulsed nanosecond optical parametric oscillators: experimental investigation and numerical analysis," *J. Opt. Soc. Am. B* **13**, 2484–2497 (1996).
3. G. Arisholm, "Quantum noise initiation and macroscopic fluctuations in optical parametric oscillators," *J. Opt. Soc. Am. B* **16**, 117–127 (1999).
4. L. Ledezma, R. Sekine, Q. Guo, *et al.*, "Intense optical parametric amplification in dispersion-engineered nanophotonic lithium niobate waveguides," *Optica* **9**, 303–308 (2022).
5. K. Thyagarajan and A. Ghatak, "Fiber and guided wave optics | nonlinear optics," in *Encyclopedia of Modern Optics*, R. D. Guenther, ed. (Elsevier, Oxford, 2005), pp. 472–486.
6. D. Zhu, L. Shao, M. Yu, *et al.*, "Integrated photonics on thin-film lithium niobate," *Adv. Opt. Photonics* **13**, 242–352 (2021).
7. T. Chen, J. Sun, L. Li, and Y. Zhou, "Analysis of difference frequency generation and cascaded second-harmonic generation and difference frequency generation in lossy quasi-phase-matched semiconductor waveguides," *Opt. Commun.* **285**, 3642–3648 (2012).
